# Supplementary material for: Carbon: Scaling Trusted Payments with Untrusted Machines
Source: arXiv:2209.09580 source file (2024-08-15)
Supplement: Supplementary file 1 [file modules.tex]

\section{Server Modules}

This section discusses the modules that comprise a correct server.
Modules of a server are able to communicate among themselves.
First, we briefly discuss each module, we define module functions exposed to other modules and present the communication pattern between the modules.

\para{Master Module}
Master module represents the main module of a server.
This module is responsible for processing transactions and join/leave requests.

\begin{lstlisting}[
  caption={Master Module},
  label={lst:master_module},
  escapechar=?]
?\textbf{Master Module:}?
    ?\textcolor{blue}{Local variables:}?
        View ?$\mathit{current\_view}$?
        Bool ?$\mathit{processing}$?
        
    ?\textcolor{blue}{Local notifications:}?
        - <Install, View ?$v$?>: the server installs view ?$v$?.
        - <Proposed_Membership, View ?$v$?>: the server proposes a ?new? system membership for view ?$v$?.
        - <Joined>: the server joins.
        - <Left>: the server leaves.
        - <Stop_Processing, View ?$v$?>: the server stops processing transactions for view ?$v$?.
\end{lstlisting}

\para{Storage Module}
Storage module is the module used for storing acknowledged and committed transactions, as well as received protocol messages.

\begin{lstlisting}[
  caption={Storage Module},
  label={lst:storage_module},
  escapechar=?]
?\textbf{Storage Module:}?
    ?\textcolor{blue}{Local variables:}?
        Set(Transaction) ?$\mathit{acknowledged\_transactions}$?
        Set(Transaction) ?$\mathit{committed\_transactions}$?
        State ?$\mathit{current\_state}$?
        Set(Message) ?$\mathit{waiting\_messages}$?
        Set(Message) ?$\mathit{install\_messages}$?
        Sequence ?$\mathit{history}$?
        
        Set(Change) ?$\mathit{admissible}$?
        Set(Change) ?$\mathit{requested}$?
\end{lstlisting}

\para{Reconfiguration Module}
Reconfiguration module is the module used for ensuring that the server updates its $\mathit{current\_view}$ variable to reflect system membership changes.

\begin{lstlisting}[
  caption={Reconfiguration Module},
  label={lst:reconfiguration_module},
  escapechar=?]
?\textbf{Reconfiguration Module:}?
    ?\textcolor{blue}{Local requests:}?
        - <Join, Join_Proof ?$\sigma$?>: the server requests to join (?i.e.,? to transit to the joined state) with the proof ?$\sigma$?.
        - <Leave>: the server requests to leave (?i.e.,? to transit to the halted state).
\end{lstlisting}
